# Supplementary material for: PIXAL: Anomaly Reasoning with Visual Analytics
Source: arXiv:2205.11004 source file (2022-05-23)
Supplement: Supplementary file 1 [file appendix.tex]

\section*{Appendix}

\sys supports the analysts' workflow presented in figure
% \ref{fig:analystWorkflowAndRequirements}
2 by finding combinations of data slices or predicates that present a high Bayesian hypothesis score. The process of generating such high scored predicates is explained visually in figure \ref{fig:explanation}. The \alg starts with the analysts inputting their data and the corresponding anomaly scores. Under the hood, this algorithm splits each feature into intervals (if the feature is continuous) or bins (if it's categorical). We call these base predicates $I_{j}$, and an example of a base predicate would be $\text{city} = \text{'Boston'}$. Then, for each $I_{j}$, we perform a recursive process where we expand it to include another base predicate, e.g. now the expanded predicate would be $\text{city} = \text{'Boston'}$ \emph{and} $6.6 < \text{precipitation} < 7.6$.

Moving forward in the process, the Bayesian hypothesis score is computed on the original predicate and the expanded one. If the original predicate had a higher score, then we keep only the original predicate and we proceed following two stopping conditions: try expanding it with other base predicates until we find a combination that improves the above mentioned score, \emph{or} until there are no other base predicates, which it means that we can add this predicate to the list of selected predicates. Once the recursive algorithm has done a pass through all the base predicates and all the combinations and stores the ones with the highest Bayesian hypothesis score, the algorithm does a final pass through the generated predicates. In this final pass merging is being performed, that is, if two predicates contain the same clauses but in a different order, then one of those two predicates is being discarded.
%

% \subsection{System Overview}
\begin{figure}
\centering
%\vspace{-1em}
\includegraphics[width=\linewidth]{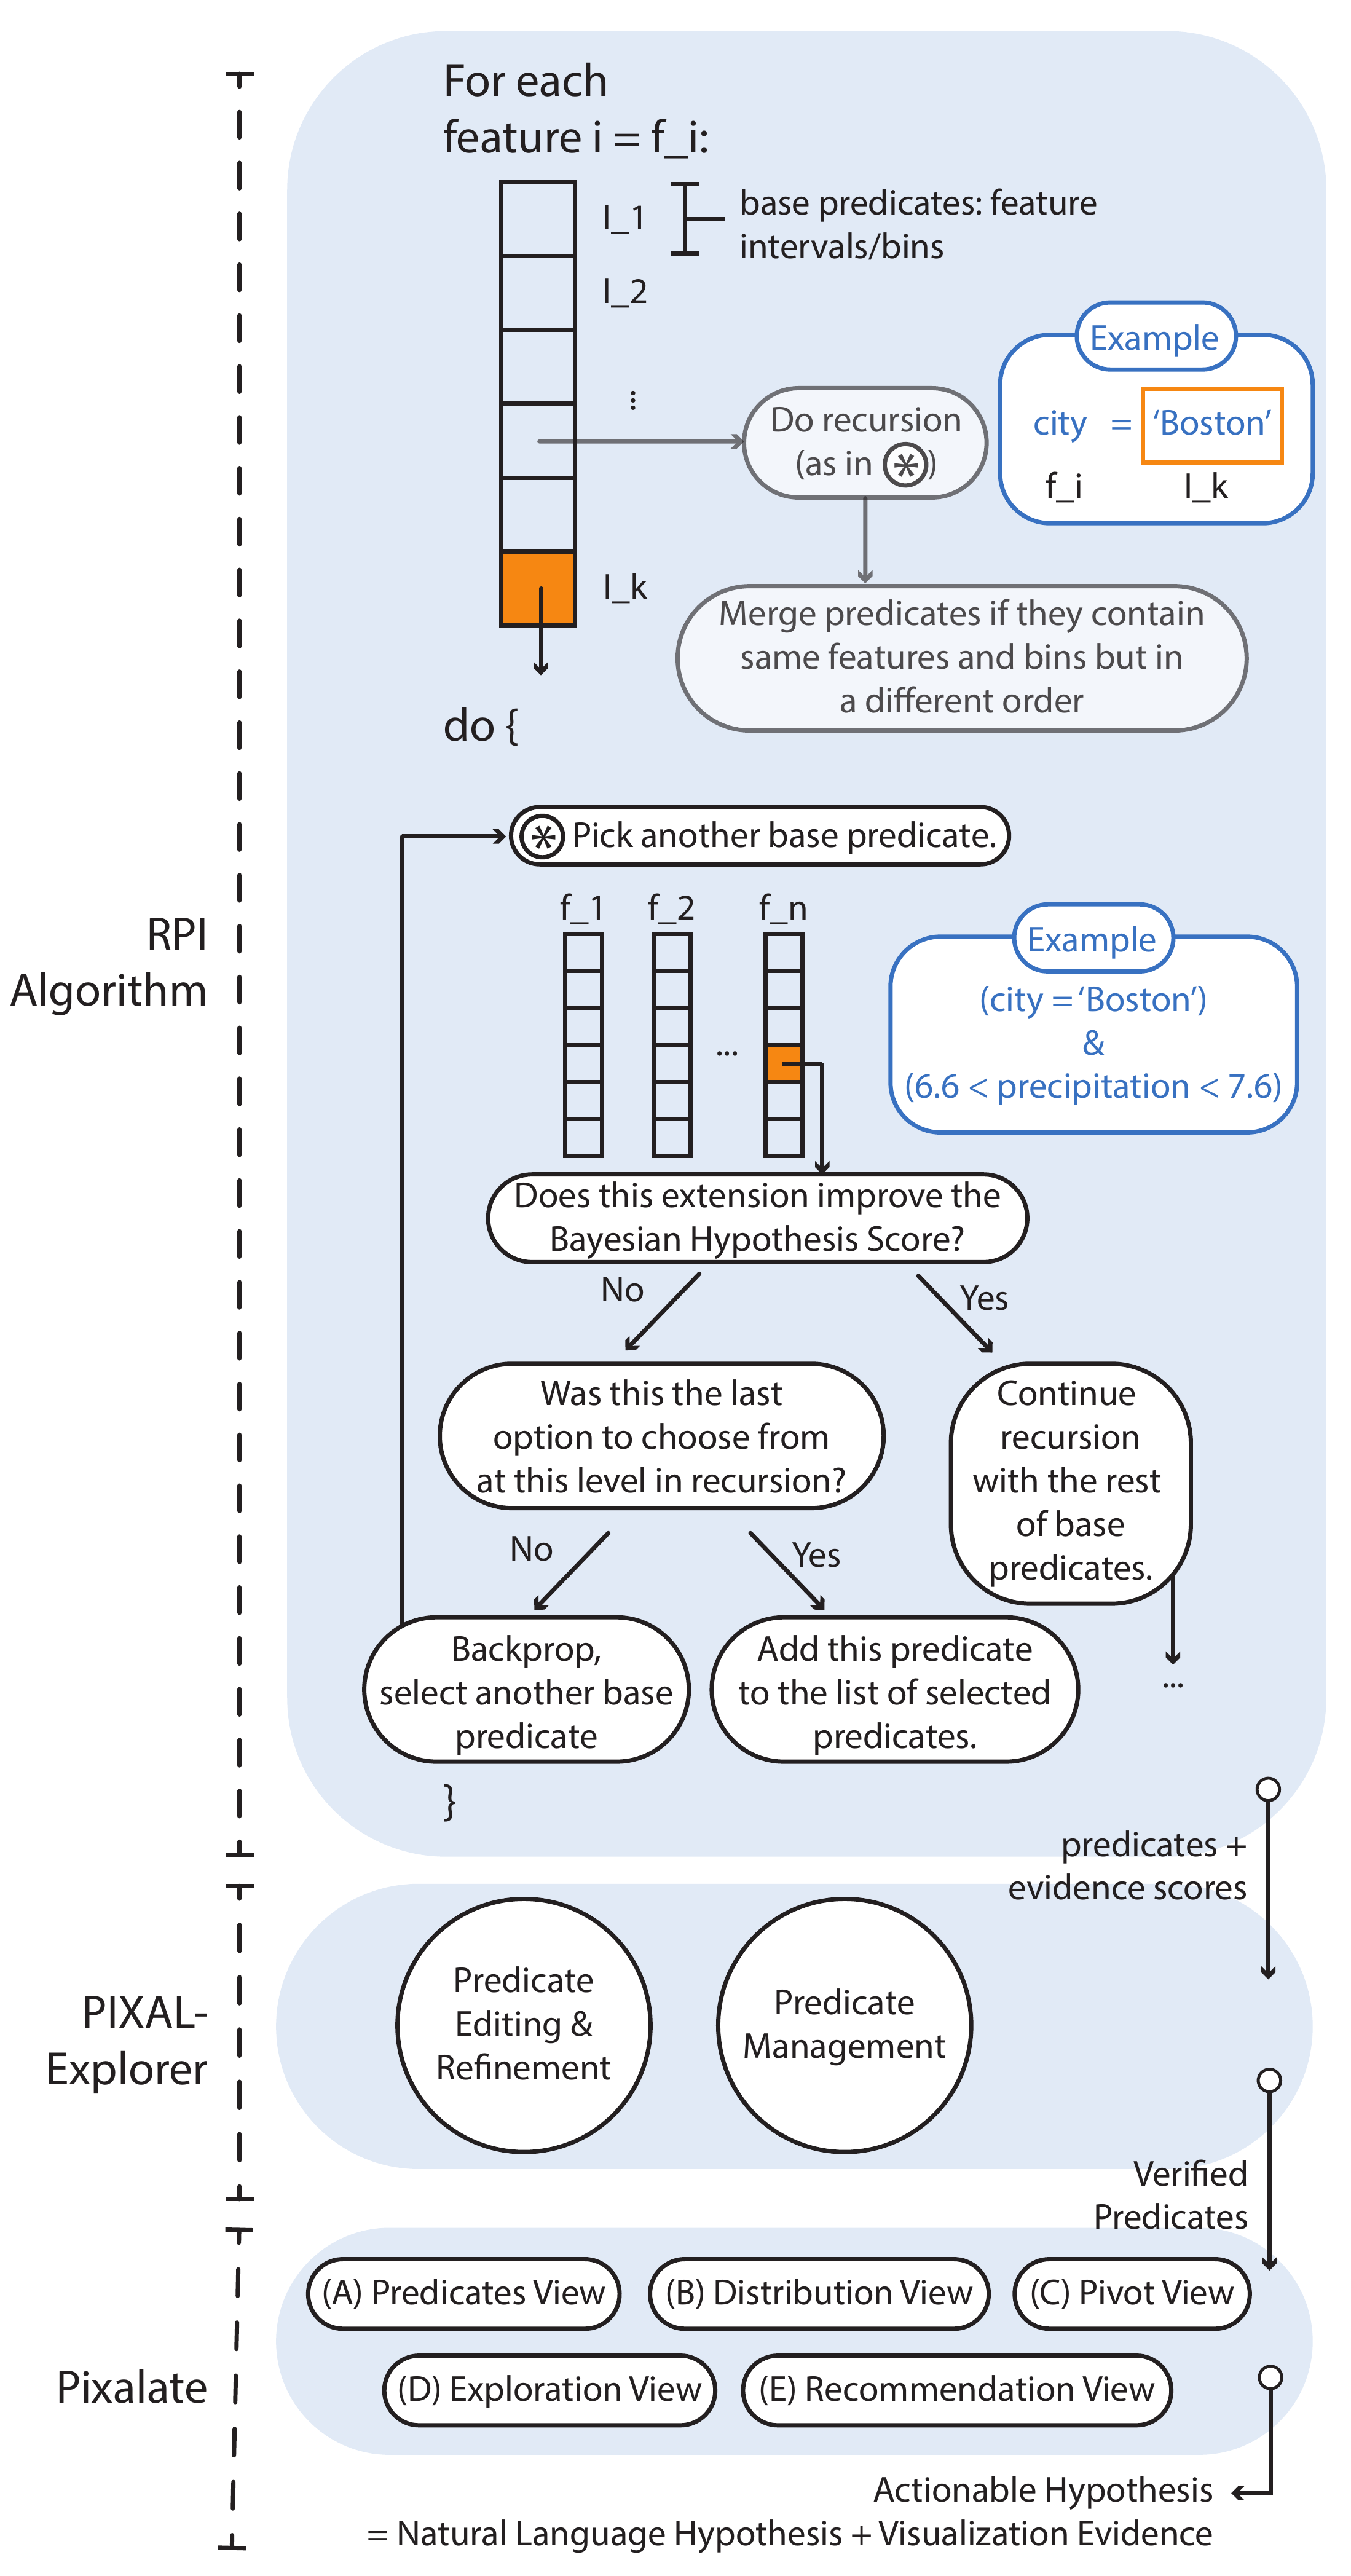}
\caption{Diagram of \sys's 3 main components, emphasizing the \alg's inner workings.}
%\vspace{-2em}
\label{fig:explanation}
\end{figure}
